# Supplementary material for: MultiHaystack: Benchmarking Multimodal Retrieval and Reasoning over 40K Images, Videos, and Documents
Source: arXiv:2603.05697 source file (2026-03-05)
Supplement: Supplementary file 1 [file single_modality.tex]

\section{Single-modality experimental results}

\begin{table*}[!ht]
\centering
\caption{\textbf{Comparison of retrieval performance under single-modality (main row) and cross-modality {\color{gray}(gray row)} settings.} Each model's main row reports single-modality retrieval scores (query and corpus belong to the same modality), while the gray row below shows its cross-modal results (e.g., text-to-video). Overall scores are shown for cross-modal only. This layout highlights how modality mismatch affects retrieval performance.}
\label{tab:retrieval_singlemodality}
\resizebox{\textwidth}{!}{%
\setlength{\tabcolsep}{5pt}

\begin{tabular}{l ccc ccc ccc ccc}
\toprule
\multirow{2}{*}{\textbf{Model}} &
\multicolumn{3}{c}{\textbf{Video}} &
\multicolumn{3}{c}{\textbf{Image}} &
\multicolumn{3}{c}{\textbf{Document}} &
\multicolumn{3}{c}{\textbf{Overall}} \\
\cmidrule(lr){2-4} \cmidrule(lr){5-7} \cmidrule(lr){8-10} \cmidrule(lr){11-13}
& \textbf{R@1} & \textbf{R@3} & \textbf{R@5}
& \textbf{R@1} & \textbf{R@3} & \textbf{R@5}
& \textbf{R@1} & \textbf{R@3} & \textbf{R@5}
& \textbf{R@1} & \textbf{R@3} & \textbf{R@5} \\
\midrule

CLIP & 56.19 & 78.10 & 80.00 & 30.25 & 40.88 & 44.34 & 38.76 & 51.67 & 53.59 & 36.28 & 49.13 & 51.94 \\
\rowcolor{gray!10} & {\color{gray}26.67} & {\color{gray}40.00} & {\color{gray}51.43} & {\color{gray}21.71} & {\color{gray}31.64} & {\color{gray}34.87} & {\color{gray}34.93} & {\color{gray}46.89} & {\color{gray}48.80} & {\color{gray}26.10} & {\color{gray}37.08} & {\color{gray}41.10} \\

SigLIP2 & \textbf{63.81} & \textbf{83.81} & \textbf{91.43} & \textbf{44.11} & 53.12 & 58.66 & 61.72 & 70.33 & 75.12 & \textbf{51.81} & 62.25 & 67.87 \\
\rowcolor{gray!10} & {\color{gray}40.00} & {\color{gray}60.00} & {\color{gray}74.29} & {\color{gray}32.10} & {\color{gray}40.88} & {\color{gray}45.27} & {\color{gray}59.81} & {\color{gray}68.42} & {\color{gray}72.73} & {\color{gray}40.96} & {\color{gray}51.27} & {\color{gray}57.03} \\

OpenCLIP & 60.00 & 74.29 & 78.10 & 25.40 & 35.80 & 42.26 & 32.06 & 42.58 & 47.85 & 32.13 & 43.11 & 48.86 \\
\rowcolor{gray!10} & {\color{gray}38.10} & {\color{gray}56.19} & {\color{gray}62.86} & {\color{gray}19.40} & {\color{gray}27.94} & {\color{gray}32.33} & {\color{gray}28.71} & {\color{gray}36.84} & {\color{gray}43.06} & {\color{gray}24.63} & {\color{gray}34.40} & {\color{gray}39.63} \\

Jina-Clip-V1 & 42.86 & 59.05 & 67.62 & 13.39 & 19.17 & 22.40 & 17.70 & 21.05 & 22.97 & 18.74 & 25.30 & 28.92 \\
\rowcolor{gray!10} & {\color{gray}21.90} & {\color{gray}38.10} & {\color{gray}47.62} & {\color{gray}7.39} & {\color{gray}10.16} & {\color{gray}12.93} & {\color{gray}16.75} & {\color{gray}21.05} & {\color{gray}22.49} & {\color{gray}12.05} & {\color{gray}17.14} & {\color{gray}20.48} \\

Jina-Clip-V2 & 36.19 & 56.19 & 76.19 & 27.25 & 42.73 & 48.04 & 41.63 & 51.67 & 56.46 & 32.53 & 47.12 & 54.35 \\
\rowcolor{gray!10} & {\color{gray}20.00} & {\color{gray}30.48} & {\color{gray}35.24} & {\color{gray}11.78} & {\color{gray}21.02} & {\color{gray}25.17} & {\color{gray}40.67} & {\color{gray}51.67} & {\color{gray}55.98} & {\color{gray}21.02} & {\color{gray}30.92} & {\color{gray}35.21} \\

Nomic-Embed-Vision & 38.10 & 54.29 & 60.95 & 8.78 & 12.01 & 13.63 & 10.53 & 13.88 & 16.27 & 13.39 & 18.47 & 21.02 \\
\rowcolor{gray!10} & {\color{gray}25.71} & {\color{gray}40.00} & {\color{gray}42.86} & {\color{gray}5.31} & {\color{gray}7.39} & {\color{gray}8.78} & {\color{gray}9.09} & {\color{gray}12.92} & {\color{gray}13.88} & {\color{gray}9.24} & {\color{gray}13.52} & {\color{gray}14.99} \\

E5-V & 62.86 & 81.90 & 83.81 & 43.19 & \textbf{68.36} & \textbf{73.44} & 60.77 & \textbf{71.29} & \textbf{76.08} & 50.87 & \textbf{71.08} & \textbf{75.64} \\
\rowcolor{gray!10} & {\color{gray}34.29} & {\color{gray}51.43} & {\color{gray}60.95} & {\color{gray}33.49} & {\color{gray}55.20} & {\color{gray}62.82} & {\color{gray}59.33} & {\color{gray}70.33} & {\color{gray}75.12} & {\color{gray}40.83} & {\color{gray}58.90} & {\color{gray}66.00} \\

MM-Embed & 60.95 & 80.00 & 87.62 & 43.65 & 64.43 & 67.21 & \textbf{62.68} & 67.46 & 75.60  & 51.41 & 67.47 & 72.42 \\
\rowcolor{gray!10} & {\color{gray}37.14} & {\color{gray}47.62} & {\color{gray}55.24} & {\color{gray}31.41} & {\color{gray}43.65} & {\color{gray}51.27} & {\color{gray}53.59} & {\color{gray}62.68} & {\color{gray}70.81} & {\color{gray}38.42} & {\color{gray}49.53} & {\color{gray}57.30} \\

\bottomrule
\end{tabular}}
\end{table*}

\begin{table*}[!ht]
  \centering
  \caption{\textbf{VQA performance across single-modality corpora.} Each model answers questions using the Recall@5 items retrieved from the single-modality. {\color{gray}Gray} font indicates Recall@5 from cross-modality retrieval evaluations, offering insight into contextual grounding performance under retrieval-augmented settings.}
  \label{tab:vqa_singlemodality}
  \resizebox{0.75\textwidth}{!}{%
    \setlength{\tabcolsep}{6pt}%
    \begin{tabular}{l c c c c}
      \toprule
      \textbf{Model} & \textbf{Video} & \textbf{Image} & \textbf{Document} & \textbf{Overall} \\
      \midrule
      Ola      
      & 22.86 {\color{gray}\scriptsize(14.29)} 
      & 31.41 {\color{gray}\scriptsize(20.09)} 
      & 44.98 {\color{gray}\scriptsize(36.36)} 
      & 34.00 {\color{gray}\scriptsize(23.83)} \\

      InternVL-3 
      & 20.95 {\color{gray}\scriptsize(17.14)} 
      & 38.80 {\color{gray}\scriptsize(29.33)} 
      & 51.67 {\color{gray}\scriptsize(49.28)} 
      & 39.89 {\color{gray}\scriptsize(33.29)} \\

      Qwen2-VL  
      & 18.10 {\color{gray}\scriptsize(16.19)} 
      & 24.94 {\color{gray}\scriptsize(16.86)} 
      & 22.49 {\color{gray}\scriptsize(19.62)} 
      & 23.29 {\color{gray}\scriptsize(17.54)} \\

      Gemini-2.5-Flash
      & 61.90 {\color{gray}\scriptsize(52.38)} 
      & 44.57 {\color{gray}\scriptsize(35.10)} 
      & 58.37 {\color{gray}\scriptsize(56.94)} 
      & 50.87 {\color{gray}\scriptsize(43.64)} \\

      GPT-5   
      & \textbf{67.62} {\color{gray}\scriptsize(60.00)} 
      & \textbf{52.66} {\color{gray}\scriptsize(43.19)} 
      & \textbf{70.81} {\color{gray}\scriptsize(64.11)} 
      & \textbf{59.84} {\color{gray}\scriptsize(51.41)} \\
      \bottomrule
    \end{tabular}%
  }
\end{table*}

\noindent \textbf{Retrieval performance within single-modality corpus.}
\Cref{tab:retrieval_singlemodality} compares Recall@K under single-modality retrieval (main rows) and cross-modality retrieval (gray rows) for video, image, and document data. In the single-modality setting, SigLIP2 attains the best video results (R@1 = 63.81, R@5 = 91.43), followed closely by E5-V (62.86/83.81) and MM-Embed (60.95/87.62). For images, SigLIP2 yields the highest R@1 (44.11), while E5-V leads at higher ranks (R@3 = 68.36, R@5 = 73.44), with MM-Embed competitive at R@1 = 43.65. For documents, MM-Embed achieves the top R@1 (62.68), with SigLIP2 (61.72) and E5-V (60.77) close behind; E5-V delivers the strongest R@3/R@5 (71.29/76.08). The gray rows quantify performance when the query and corpus differ in modality. Aggregating across modalities (Overall column), SigLIP2 is the best cross-modal retriever (R@1/R@3/R@5 = 51.81/62.25/67.87), followed by E5-V (40.83/58.90/66.00) and MM-Embed (38.42/49.53/57.30). By modality, cross-modal video retrieval is led by SigLIP2 (R@1 = 40.00; R@5 = 74.29); cross-modal image retrieval is strongest for E5-V (R@1 = 33.49; R@5 = 62.82); and cross-modal document retrieval is shared between SigLIP2 (best R@1 = 59.81) and E5-V (best R@3/R@5 = 70.33/75.12).

When comparing the single-modality results (main rows) with their corresponding cross-modal counterparts (gray rows) in \cref{tab:retrieval_singlemodality}, it becomes evident that retrieval performance is generally stronger when both the query and the corpus originate from the same modality.
This contrast reflects the increased difficulty of cross-modal retrieval, where the system must align semantically diverse representations across different input formats.
The gap is especially pronounced in video retrieval tasks, where challenges stem from complex temporal layouts.
These results highlight the importance of strong unimodal encoders and suggest that continued progress in modality-specific representation learning is essential for improving overall multimodal retrieval performance.

\noindent \textbf{VQA performance within single-modality corpus.} \Cref{tab:vqa_singlemodality} reports VQA accuracy on single-modality corpora (video, image, document) using the Recall@5 items retrieved from the same modality; gray numbers in parentheses show the corresponding Recall@5 under cross-modal retrieval. Overall, GPT-5 is the strongest system, achieving the highest scores in all three modalities—67.62 on video, 52.66 on images, and 70.81 on documents—yielding an overall accuracy of 59.84. Gemini-2.5-Flash is the next best performer (61.90/44.57/58.37; overall 50.87). Among the remaining models, InternVL-3 (20.95/38.80/51.67; overall 39.89) outperforms Ola (22.86/31.41/44.98; overall 34.00) and Qwen2-VL (18.10/24.94/22.49; overall 23.29). For most models, document VQA yields the highest single-modality accuracy (e.g., GPT-5: 70.81; InternVL-3: 51.67; Ola: 44.98), while video scores vary more sharply across systems.

The gray values highlight the effect of using cross-modal retrieval to form the evidence set. Accuracy consistently declines relative to the single-modality condition, and the overall drops are 8.43 points for GPT-5 (59.84$\to$51.41), 7.23 for Gemini-2.5-Flash (50.87$\to$43.64), 6.60 for InternVL-3 (39.89$\to$33.29), 10.17 for Ola (34.00$\to$23.83), and 5.75 for Qwen2-VL (23.29$\to$17.54). By modality, the degradation is typically largest on images (e.g., $-9.47$ for GPT-5 and Gemini-2.5-Flash) and smallest on documents (e.g., $-1.43$ for Gemini-2.5-Flash; $-2.39$ for InternVL-3), indicating that document-grounded reasoning is relatively robust to modality mismatch, whereas image-grounded reasoning is more sensitive. The ranking of methods remains stable across settings, with GPT-5 $>$ Gemini-2.5-Flash $>$ InternVL-3 $>$ Ola $>$ Qwen2-VL both per-modality (up to minor variations) and in the overall metric.
