# Supplementary material for: MultiHaystack: Benchmarking Multimodal Retrieval and Reasoning over 40K Images, Videos, and Documents
Source: arXiv:2603.05697 source file (2026-03-05)
Supplement: Supplementary file 2 [file upper_bound.tex]

\section{Upper-Bound of VQA models}

\begin{table*}[!ht]
\centering
\caption{\textbf{Upper-bound analysis for VQA models.} We estimate ceilings under three evidence regimes: G@1 (Gold in Top 1)—the ground-truth positive item is given as the only context; G@5 (Gold in Top 5)—the positive item is inserted at a random position among five candidates; and R@5 (Recall@5)—the top-5 items returned by the E5-V retriever are provided as context. Reported scores reflect VQA performance conditioned on each regime. }
\label{tab:upper_bound}
\resizebox{\textwidth}{!}{%
\setlength{\tabcolsep}{6pt}%
\begin{tabular}{l ccc ccc ccc ccc}
\toprule
\multirow{2}{*}{\textbf{Model}} &
\multicolumn{3}{c}{\textbf{Video}} &
\multicolumn{3}{c}{\textbf{Image}} &
\multicolumn{3}{c}{\textbf{Document}} &
\multicolumn{3}{c}{\textbf{Overall}} \\
\cmidrule(lr){2-4}\cmidrule(lr){5-7}\cmidrule(lr){8-10}\cmidrule(lr){11-13}
& \textbf{G@1} & \textbf{G@5} & \textbf{R@5}
& \textbf{G@1} & \textbf{G@5} & \textbf{R@5}
& \textbf{G@1} & \textbf{G@5} & \textbf{R@5}
& \textbf{G@1} & \textbf{G@5} & \textbf{R@5} \\
    \midrule
Ola        & 59.05 & 48.57 & 14.29 & 46.42 & 38.11 & 20.09 & 59.33 & 51.20 & 36.36 & 51.81 & 43.24 & 23.83 \\
InternVL-3 &  63.81   & 55.24    &  17.14   &  48.50   & 40.42    & 29.33    &  64.11   &  57.89   &  49.28   & 55.02   &  47.39   & 33.29    \\
Qwen2-VL    & 54.29 &  45.71 & 16.19 & 37.18 & 30.25 &  16.86 & 49.76 & 42.58 & 19.62 & 43.11 & 35.88 & 17.54 \\
Gemini-2.5-Flash  & 85.71 & 81.90 & 52.38 & 69.52 &  47.34 & 35.10 &  79.90 & 74.16 & 56.94 & 74.70 & 59.71 & 43.64 \\
GPT-5  & \textbf{89.52} &  \textbf{85.71} & \textbf{60.00} &  \textbf{75.75} &  \textbf{59.82} & \textbf{43.19} & \textbf{87.08} & \textbf{78.47}  & \textbf{64.11}  & \textbf{80.86} & \textbf{68.67} & \textbf{51.41} \\
\bottomrule
\end{tabular}}
\end{table*}

\Cref{tab:upper_bound} decomposes performance in our cross-modal retrieval-augmented VQA into three evidence regimes with the expected ordering G@1 $\textgreater$ G@5 $\textgreater$ R@5. The G@1$\to$G@5 gap isolates robustness to distractors: G@1 supplies only the gold context and therefore reflects reasoning under perfectly curated evidence, whereas G@5 mixes the gold with four distractors and requires the model to first localize the relevant item before reasoning. The G@5$\to$R@5 gap quantifies the retrieval bottleneck: unlike G@5, which guarantees oracle recall@5=100\%, R@5 relies on the retriever’s top-5 candidates and thus its drop captures deficiencies in recall, precision, and ranking. Modality-wise, documents typically show smaller G@1$\to$G@5 drops due to explicit textual anchors, while images tend to incur larger drops because visual cues are more ambiguous. Overall, stronger LMMs reduce both gaps, indicating improved grounding and tolerance to distractors; nevertheless, the residual G@5→R@5 gap shows that end-to-end performance remains primarily constrained by retrieval quality once adequate context is available.
