# Supplementary material for: MultiHaystack: Benchmarking Multimodal Retrieval and Reasoning over 40K Images, Videos, and Documents
Source: arXiv:2603.05697 source file (2026-03-05)
Supplement: Supplementary file 3 [file llm_evaluation.tex]

% \section{Reliability of LLMs as an Automatic Judge}

% \input{iclr2026/appendix/table/llm_eval}

% Table~\ref{tab:llm_eval} shows that using GPT-4o-mini as the LLM-as-judge yields consistently high agreement with human annotations across all evaluated models. Cohen’s $\kappa$ averages $\approx$ 0.94 (with two cases at 1.00), accuracies are around 0.97, and the continuous scores correlate strongly with human judgments (Pearson r $\approx$ 0.95). Several confidence intervals even collapse to [1.000, 1.000], underscoring the stability of the judge. These results indicate that GPT-4o-mini provides a reliable and scalable substitute for manual scoring in our experiments.
