# Supplementary material for: MultiHaystack: Benchmarking Multimodal Retrieval and Reasoning over 40K Images, Videos, and Documents
Source: arXiv:2603.05697 source file (2026-03-05)
Supplement: Supplementary file 4 [file retrieval_singlemodality.tex]

\begin{table*}[!ht]
\centering
\caption{\textbf{Comparison of retrieval performance under single-modality (main row) and cross-modality {\color{gray}(gray row)} settings.} Each model's main row reports single-modality retrieval scores (query and corpus belong to the same modality), while the gray row below shows its cross-modal results (e.g., text-to-video). Overall scores are shown for cross-modal only. This layout highlights how modality mismatch affects retrieval performance.}
\label{tab:retrieval_singlemodality}
\resizebox{\textwidth}{!}{%
\setlength{\tabcolsep}{5pt}

\begin{tabular}{l ccc ccc ccc ccc}
\toprule
\multirow{2}{*}{\textbf{Model}} &
\multicolumn{3}{c}{\textbf{Video}} &
\multicolumn{3}{c}{\textbf{Image}} &
\multicolumn{3}{c}{\textbf{Document}} &
\multicolumn{3}{c}{\textbf{Overall}} \\
\cmidrule(lr){2-4} \cmidrule(lr){5-7} \cmidrule(lr){8-10} \cmidrule(lr){11-13}
& \textbf{R@1} & \textbf{R@3} & \textbf{R@5}
& \textbf{R@1} & \textbf{R@3} & \textbf{R@5}
& \textbf{R@1} & \textbf{R@3} & \textbf{R@5}
& \textbf{R@1} & \textbf{R@3} & \textbf{R@5} \\
\midrule

CLIP & 56.19 & 78.10 & 80.00 & 30.25 & 40.88 & 44.34 & 38.76 & 51.67 & 53.59 & 36.28 & 49.13 & 51.94 \\
\rowcolor{gray!10} & {\color{gray}26.67} & {\color{gray}40.00} & {\color{gray}51.43} & {\color{gray}21.71} & {\color{gray}31.64} & {\color{gray}34.87} & {\color{gray}34.93} & {\color{gray}46.89} & {\color{gray}48.80} & {\color{gray}26.10} & {\color{gray}37.08} & {\color{gray}41.10} \\

SigLIP2 & \textbf{63.81} & \textbf{83.81} & \textbf{91.43} & \textbf{44.11} & 53.12 & 58.66 & 61.72 & 70.33 & 75.12 & \textbf{51.81} & 62.25 & 67.87 \\
\rowcolor{gray!10} & {\color{gray}40.00} & {\color{gray}60.00} & {\color{gray}74.29} & {\color{gray}32.10} & {\color{gray}40.88} & {\color{gray}45.27} & {\color{gray}59.81} & {\color{gray}68.42} & {\color{gray}72.73} & {\color{gray}40.96} & {\color{gray}51.27} & {\color{gray}57.03} \\

OpenCLIP & 60.00 & 74.29 & 78.10 & 25.40 & 35.80 & 42.26 & 32.06 & 42.58 & 47.85 & 32.13 & 43.11 & 48.86 \\
\rowcolor{gray!10} & {\color{gray}38.10} & {\color{gray}56.19} & {\color{gray}62.86} & {\color{gray}19.40} & {\color{gray}27.94} & {\color{gray}32.33} & {\color{gray}28.71} & {\color{gray}36.84} & {\color{gray}43.06} & {\color{gray}24.63} & {\color{gray}34.40} & {\color{gray}39.63} \\

Jina-Clip-V1 & 42.86 & 59.05 & 67.62 & 13.39 & 19.17 & 22.40 & 17.70 & 21.05 & 22.97 & 18.74 & 25.30 & 28.92 \\
\rowcolor{gray!10} & {\color{gray}21.90} & {\color{gray}38.10} & {\color{gray}47.62} & {\color{gray}7.39} & {\color{gray}10.16} & {\color{gray}12.93} & {\color{gray}16.75} & {\color{gray}21.05} & {\color{gray}22.49} & {\color{gray}12.05} & {\color{gray}17.14} & {\color{gray}20.48} \\

Jina-Clip-V2 & 36.19 & 56.19 & 76.19 & 27.25 & 42.73 & 48.04 & 41.63 & 51.67 & 56.46 & 32.53 & 47.12 & 54.35 \\
\rowcolor{gray!10} & {\color{gray}20.00} & {\color{gray}30.48} & {\color{gray}35.24} & {\color{gray}11.78} & {\color{gray}21.02} & {\color{gray}25.17} & {\color{gray}40.67} & {\color{gray}51.67} & {\color{gray}55.98} & {\color{gray}21.02} & {\color{gray}30.92} & {\color{gray}35.21} \\

Nomic-Embed-Vision & 38.10 & 54.29 & 60.95 & 8.78 & 12.01 & 13.63 & 10.53 & 13.88 & 16.27 & 13.39 & 18.47 & 21.02 \\
\rowcolor{gray!10} & {\color{gray}25.71} & {\color{gray}40.00} & {\color{gray}42.86} & {\color{gray}5.31} & {\color{gray}7.39} & {\color{gray}8.78} & {\color{gray}9.09} & {\color{gray}12.92} & {\color{gray}13.88} & {\color{gray}9.24} & {\color{gray}13.52} & {\color{gray}14.99} \\

E5-V & 62.86 & 81.90 & 83.81 & 43.19 & \textbf{68.36} & \textbf{73.44} & 60.77 & \textbf{71.29} & \textbf{76.08} & 50.87 & \textbf{71.08} & \textbf{75.64} \\
\rowcolor{gray!10} & {\color{gray}34.29} & {\color{gray}51.43} & {\color{gray}60.95} & {\color{gray}33.49} & {\color{gray}55.20} & {\color{gray}62.82} & {\color{gray}59.33} & {\color{gray}70.33} & {\color{gray}75.12} & {\color{gray}40.83} & {\color{gray}58.90} & {\color{gray}66.00} \\

MM-Embed & 60.95 & 80.00 & 87.62 & 43.65 & 64.43 & 67.21 & \textbf{62.68} & 67.46 & 75.60  & 51.41 & 67.47 & 72.42 \\
\rowcolor{gray!10} & {\color{gray}37.14} & {\color{gray}47.62} & {\color{gray}55.24} & {\color{gray}31.41} & {\color{gray}43.65} & {\color{gray}51.27} & {\color{gray}53.59} & {\color{gray}62.68} & {\color{gray}70.81} & {\color{gray}38.42} & {\color{gray}49.53} & {\color{gray}57.30} \\

\bottomrule
\end{tabular}}
\end{table*}
