# Supplementary material for: MultiHaystack: Benchmarking Multimodal Retrieval and Reasoning over 40K Images, Videos, and Documents
Source: arXiv:2603.05697 source file (2026-03-05)
Supplement: Supplementary file 5 [file upper_bound.tex]

\begin{table*}[!ht]
\centering
\caption{\textbf{Upper-bound analysis for VQA models.} We estimate ceilings under three evidence regimes: G@1 (Gold in Top 1)—the ground-truth positive item is given as the only context; G@5 (Gold in Top 5)—the positive item is inserted at a random position among five candidates; and R@5 (Recall@5)—the top-5 items returned by the E5-V retriever are provided as context. Reported scores reflect VQA performance conditioned on each regime. }
\label{tab:upper_bound}
\resizebox{\textwidth}{!}{%
\setlength{\tabcolsep}{6pt}%
\begin{tabular}{l ccc ccc ccc ccc}
\toprule
\multirow{2}{*}{\textbf{Model}} &
\multicolumn{3}{c}{\textbf{Video}} &
\multicolumn{3}{c}{\textbf{Image}} &
\multicolumn{3}{c}{\textbf{Document}} &
\multicolumn{3}{c}{\textbf{Overall}} \\
\cmidrule(lr){2-4}\cmidrule(lr){5-7}\cmidrule(lr){8-10}\cmidrule(lr){11-13}
& \textbf{G@1} & \textbf{G@5} & \textbf{R@5}
& \textbf{G@1} & \textbf{G@5} & \textbf{R@5}
& \textbf{G@1} & \textbf{G@5} & \textbf{R@5}
& \textbf{G@1} & \textbf{G@5} & \textbf{R@5} \\
    \midrule
Ola        & 59.05 & 48.57 & 14.29 & 46.42 & 38.11 & 20.09 & 59.33 & 51.20 & 36.36 & 51.81 & 43.24 & 23.83 \\
InternVL-3 &  63.81   & 55.24    &  17.14   &  48.50   & 40.42    & 29.33    &  64.11   &  57.89   &  49.28   & 55.02   &  47.39   & 33.29    \\
Qwen2-VL    & 54.29 &  45.71 & 16.19 & 37.18 & 30.25 &  16.86 & 49.76 & 42.58 & 19.62 & 43.11 & 35.88 & 17.54 \\
Gemini-2.5-Flash  & 85.71 & 81.90 & 52.38 & 69.52 &  47.34 & 35.10 &  79.90 & 74.16 & 56.94 & 74.70 & 59.71 & 43.64 \\
GPT-5  & \textbf{89.52} &  \textbf{85.71} & \textbf{60.00} &  \textbf{75.75} &  \textbf{59.82} & \textbf{43.19} & \textbf{87.08} & \textbf{78.47}  & \textbf{64.11}  & \textbf{80.86} & \textbf{68.67} & \textbf{51.41} \\
\bottomrule
\end{tabular}}
\end{table*}
