# Supplementary material for: MultiHaystack: Benchmarking Multimodal Retrieval and Reasoning over 40K Images, Videos, and Documents
Source: arXiv:2603.05697 source file (2026-03-05)
Supplement: Supplementary file 6 [file vqa_singlemodality.tex]

\begin{table*}[!ht]
  \centering
  \caption{\textbf{VQA performance across single-modality corpora.} Each model answers questions using the Recall@5 items retrieved from the single-modality. {\color{gray}Gray} font indicates Recall@5 from cross-modality retrieval evaluations, offering insight into contextual grounding performance under retrieval-augmented settings.}
  \label{tab:vqa_singlemodality}
  \resizebox{0.75\textwidth}{!}{%
    \setlength{\tabcolsep}{6pt}%
    \begin{tabular}{l c c c c}
      \toprule
      \textbf{Model} & \textbf{Video} & \textbf{Image} & \textbf{Document} & \textbf{Overall} \\
      \midrule
      Ola      
      & 22.86 {\color{gray}\scriptsize(14.29)} 
      & 31.41 {\color{gray}\scriptsize(20.09)} 
      & 44.98 {\color{gray}\scriptsize(36.36)} 
      & 34.00 {\color{gray}\scriptsize(23.83)} \\

      InternVL-3 
      & 20.95 {\color{gray}\scriptsize(17.14)} 
      & 38.80 {\color{gray}\scriptsize(29.33)} 
      & 51.67 {\color{gray}\scriptsize(49.28)} 
      & 39.89 {\color{gray}\scriptsize(33.29)} \\

      Qwen2-VL  
      & 18.10 {\color{gray}\scriptsize(16.19)} 
      & 24.94 {\color{gray}\scriptsize(16.86)} 
      & 22.49 {\color{gray}\scriptsize(19.62)} 
      & 23.29 {\color{gray}\scriptsize(17.54)} \\

      Gemini-2.5-Flash
      & 61.90 {\color{gray}\scriptsize(52.38)} 
      & 44.57 {\color{gray}\scriptsize(35.10)} 
      & 58.37 {\color{gray}\scriptsize(56.94)} 
      & 50.87 {\color{gray}\scriptsize(43.64)} \\

      GPT-5   
      & \textbf{67.62} {\color{gray}\scriptsize(60.00)} 
      & \textbf{52.66} {\color{gray}\scriptsize(43.19)} 
      & \textbf{70.81} {\color{gray}\scriptsize(64.11)} 
      & \textbf{59.84} {\color{gray}\scriptsize(51.41)} \\
      \bottomrule
    \end{tabular}%
  }
\end{table*}
